# Supplementary material for: Raman Signal Extraction from CARS Spectra Using a Learned-Matrix Representation of the Discrete Hilbert Transform
Source: arXiv:2204.00666 source file (2022-06-23)
Supplement: Supplementary file 2 [file osa-supplemental-document-template.tex]

\documentclass[9pt]{osa-supplemental-document}
\setboolean{shortarticle}{false}

\title{Title of primary manuscript: supplemental document}
\author{} %leave this blank
%% DO NOT ADD AUTHOR INFORMATION HERE; IT WILL BE ADDED DURING PRODUCTION

\begin{abstract}
This template can be used to prepare a supplementary document for inclusion with submission to Optica Publishing Group’s journals.  This document, which may include supplementary information such as expanded descriptions of materials and methods, will be published as a PDF linked to the primary article. The supplemental file should only present information that would be useful and worthwhile for the reader, for example, details that would be necessary to reproduce an experiment. The article, however, must be coherent without the supplemental PDF file.  Please see the \href{https://opg.optica.org/submit/style/supplementary_materials.cfm}{Author Guidelines for Supplementary Materials} for more information. Supplementary documents are not copyedited and so should be prepared carefully with the template provided. Note that a coversheet with final article title, author block, publication date, journal branding, and other details will be added to your supplemental document during production. Do not include such details directly in this document.  Note that this template can be run from your own \TeX\ system or within the cloud-based \href{https://www.overleaf.com}{Overleaf} system.
\end{abstract}

\setboolean{displaycopyright}{false} %copyright statement should not display in the  supplementary document

\begin{document}

\maketitle

\section{Introduction}

This template is designed to assist with creating a supplemental document to accompany an article in an Optica Publishing Group journal. This template contains example content to help you create your document, and you may use this template as a visual guide. The sections below show examples of different components and styles.


\section{Numbering Items in the Supplementary Document}

The supplementary materials document may contain additional figures, tables, equations, etc. Such items should be numbered, with an uppercase “S” to identify them as supplementary. For example, number the first figure in the supplementary document “Fig. S1”; the first table “Table S1”; etc.

This template has been designed to automatically format these components with this styling, but we include the naming convention here for reference.

\subsection*{Naming Convention for Countable Items}

\begin{condenseditemize}
\item[] Algorithm S1
\item[] Equation (S1)
\item[] Figure S1
\item[] Media S1
\item[] Table S1
\end{condenseditemize}


\section{Figures and Tables}
Figures and Tables should be labeled and referenced in the standard way using the \verb|\label{}| and \verb|\ref{}| commands.

\subsection{Sample Figure}

Figure \ref{fig:false-color} shows an example figure.

\begin{figure}[htbp]
\centering
\fbox{\includegraphics[width=.6\linewidth]{sample}}
\caption{False-color image, where each pixel is assigned to one of seven reference spectra.}
\label{fig:false-color}
\end{figure}

\subsection{Sample Table}

Table \ref{tab:shape-functions} shows an example table. 

\begin{table}[htbp]
\centering
\caption{\bf Shape Functions for Quadratic Line Elements}
\begin{tabular}{ccc}
\hline
local node & $\{N\}_m$ & $\{\Phi_i\}_m$ $(i=x,y,z)$ \\
\hline
$m = 1$ & $L_1(2L_1-1)$ & $\Phi_{i1}$ \\
$m = 2$ & $L_2(2L_2-1)$ & $\Phi_{i2}$ \\
$m = 3$ & $L_3=4L_1L_2$ & $\Phi_{i3}$ \\
\hline
\end{tabular}
  \label{tab:shape-functions}
\end{table}

\section{Sample Equation}

Let $X_1, X_2, \ldots, X_n$ be a sequence of independent and identically distributed random variables with $\text{E}[X_i] = \mu$ and $\text{Var}[X_i] = \sigma^2 < \infty$, and let
\begin{equation}
S_n = \frac{X_1 + X_2 + \cdots + X_n}{n}
      = \frac{1}{n}\sum_{i}^{n} X_i
\label{eq:refname1}
\end{equation}
denote their mean. Then as $n$ approaches infinity, the random variables $\sqrt{n}(S_n - \mu)$ converge in distribution to a normal $\mathcal{N}(0, \sigma^2)$.

\section{Sample Algorithm}

Algorithms can be included using the commands as shown in algorithm \ref{alg:euclid}.

\begin{algorithm}
\caption{Euclid’s algorithm}\label{alg:euclid}
\begin{algorithmic}[1]
\Procedure{Euclid}{$a,b$}\Comment{The g.c.d. of a and b}
\State $r\gets a\bmod b$
\While{$r\not=0$}\Comment{We have the answer if r is 0}
\State $a\gets b$
\State $b\gets r$
\State $r\gets a\bmod b$
\EndWhile\label{euclidendwhile}
\State \textbf{return} $b$\Comment{The gcd is b}
\EndProcedure
\end{algorithmic}
\end{algorithm}

\section*{Media}

The supplemental document may contain linked objects such as video, 2D, 3D, and machine-readable data files. Please see the \href{https://opg.optica.org/submit/style/supplementary_materials.cfm}{Author Guidelines for Supplementary Materials} for more information. Such files should be cited in the supplementary document as in the primary document but using the naming convention described above.

\section*{References} 

The supplementary materials document may contain a reference list. The reference list should follow our citation style and should be checked carefully, since staff will not be performing any copyediting. You may add citations manually or use BibTeX. See \cite{Zhang:14}.

Citations that are relevant to the primary manuscript and the supplementary document may be included in both places.

% Bibliography
\bibliography{sample}

%Manual citation list
%\begin{thebibliography}{1}
%\bibitem{Zhang:14}
%Y.~Zhang, S.~Qiao, L.~Sun, Q.~W. Shi, W.~Huang, %L.~Li, and Z.~Yang,
 % \enquote{Photoinduced active terahertz metamaterials with nanostructured
  %vanadium dioxide film deposited by sol-gel method,} Opt. Express \textbf{22},
  %11070--11078 (2014).
%\end{thebibliography}

\end{document}
